# Supplementary material for: Exploring External Knowledge for Accurate modeling of Visual and Language Problems
Source: arXiv:2302.08901 source file (2023-01-27)
Supplement: Supplementary file 1 [file 8_suppl.tex]

\section{Supplementary}

\subsection{More Examples on FACAD}
More examples can be found in the online anonymous website:

\url{https://github.com/anonynous10992/fashioncaptioning}.

We also showcase some examples directly in Fig~\ref{fig:sample_sup}.

\begin{figure}
% \captionsetup{font=footnotesize}
\small
\centering
\includegraphics[width=0.8\textwidth]{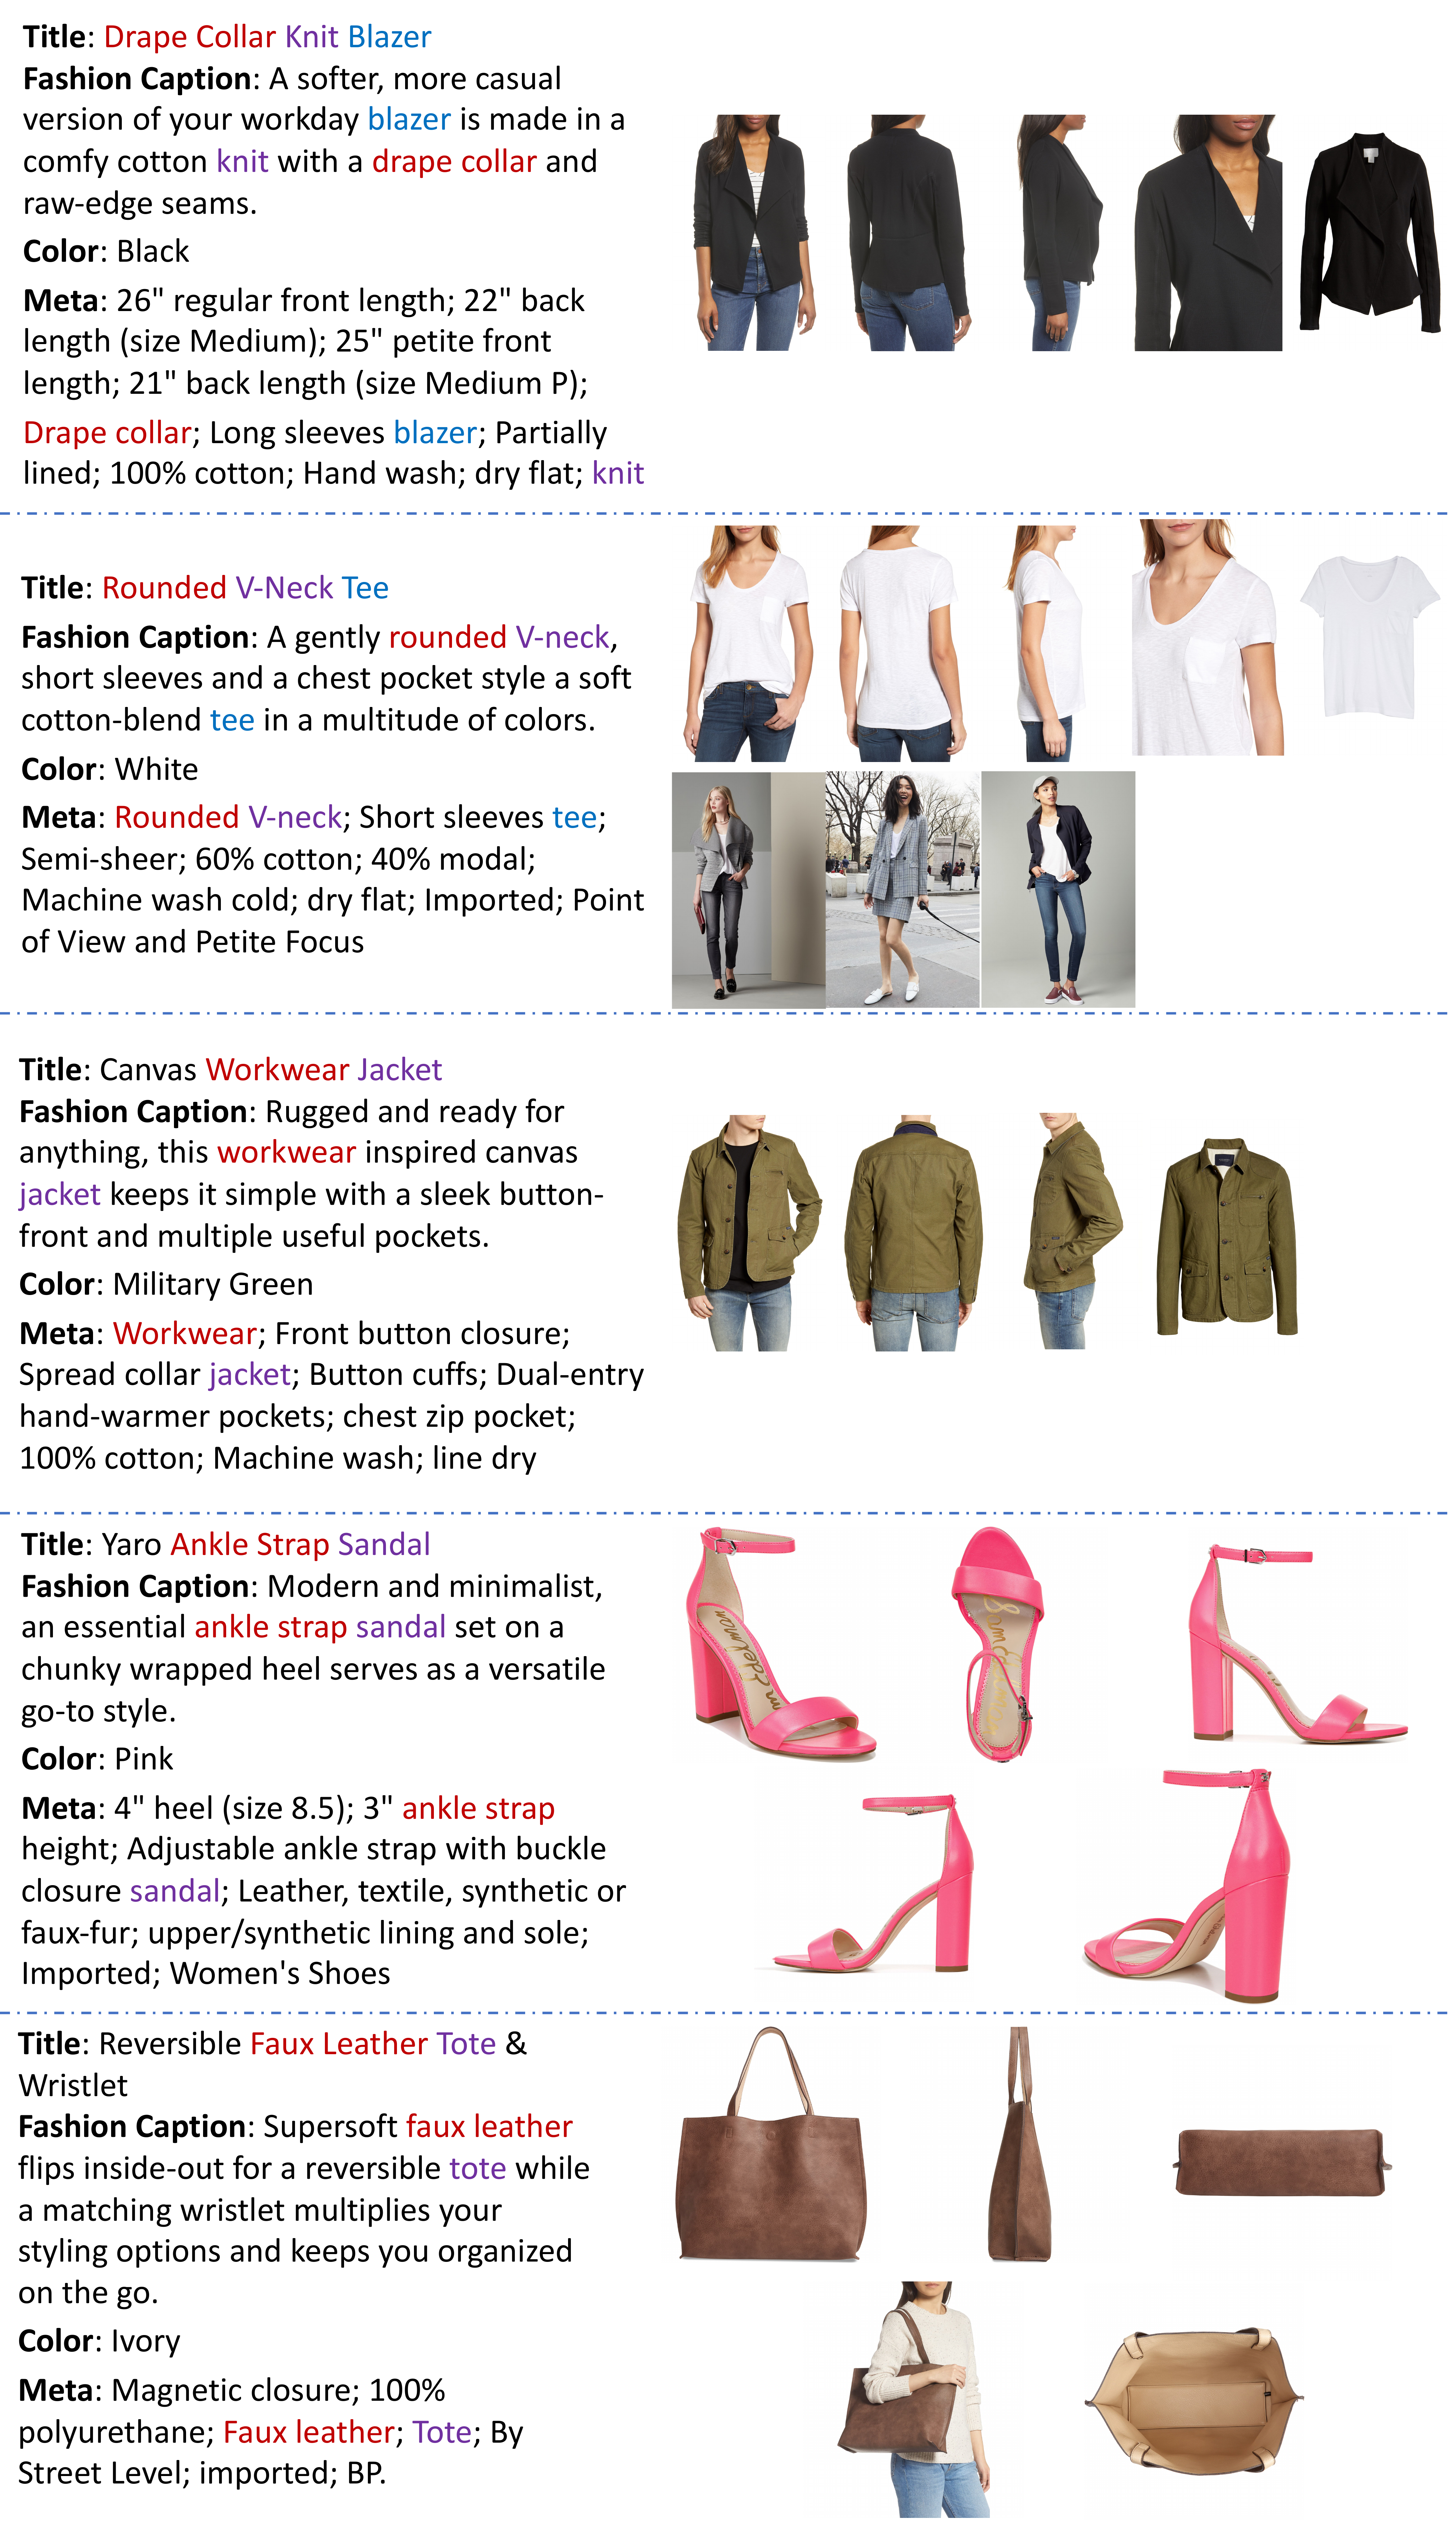}
\caption{More examples for FACAD. The images are of different perspectives, colors and scenarios (shop-street). Other information contained include a title, a description (caption) from a fashion expert, the color info and the meta info. Words in color denotes the attributes used in sentence.
}
\label{fig:sample_sup}
\vspace{-0.2in}
\end{figure}
\vspace{-0.1in}

\subsection{Categories and Attributes}
To showcase the massive categories of FACAD, we split all 74 categories into 5 subsets: top, bottom, one-piece, shoes, bags and accessories and list the 5 subsets in Table~\ref{tab:category}.

\begin{table*}[!p]
\caption{List of categories.}
\centering
\begin{tabular}{cp{10cm}cl}
%\begin{tabular}{|l|*{4}{c|}}
\toprule
%\hline
subset & categories \\
\midrule
top & tee, jacket, sweater, blouse, coat, sweatshirt, bra,  cardigan, hood, tank, blazer, top, polo, pullover, camisole, vest, turtleneck, henley, parka   \\\hline
bottom &  jeans, pants, shorts, skirt, trousers, legging, trunk, thongs, sweatpants, jeggings, tights, chinos \\\hline
one-piece & dress, gown, jumpsuit, swimsuit, bodysuit, pajamas, robe, suit, one-piece, bikini, derby, chemise  \\\hline
shoes & boot, sandal, sneaker, pump, loafer, joggers, flop, slippers, wedge, wingtip, clog  \\\hline
bags & backpack, handbag, shoulder bag, beach bag, clutch bag, tote bag, belt bag, satchels  \\\hline
accessories  & watch, hat, bracelet, gloves, necklace, glasses, wallet, rings, belt, brooches, earrings, tie, scarves \\
\bottomrule
\end{tabular}
\label{tab:category}
\end{table*}

To know more about the details of the items, we display a subset of all attributes in Table~\ref{tab:attributes}.

\begin{table*}[!p]
\caption{List of attributes.}
\centering
\begin{tabular}{p{10cm}l}
%\begin{tabular}{|l|*{4}{c|}}
\toprule
%\hline
attributes \\
\midrule

brief, paillette, slipdress, pull, park, linen, shell, sleeve, knit, maxi, dress, collar, poplin, cotton, wrap, strap, monk, logo, hood, plaid, slingback, water-resistant, fringe, stripe, sport, midi, bralette, paisley, platform, high-waist, faux-leather, front, henley, organic, track, nylon, pocket, stud, flare, thongs, waterproof, tie, neck, sparkle, graffiti, heart, chinos, cocktail, gown, silk, fill, power, brocade, sleeveless, print, skirt, solution, sequin, waffle, satin, biker, graphic, burnout, wide-leg, garment, v-neck, nursing, lace, miniskirt, blouson, chambray, step, hem, wool, straight, zip, ankle, leopard, fit, acid, cable, taper, corduroy, slide, ruffle, crop, boxer, reversible, camisole, slim, velvet, curve, dot, tank, sheath, denim, open, toe, basketball, floral, button, paperbag, trunk, wedding, bodice, chiffon, horse, stretch, crepe, twist, flag, oxford, thermal, cargo, teddy, bear, fur, patent, maternity, ponte, crewneck, classic, funnel, alpaca, blend, flannel, chukka, pinstripe, seersucker, side, bottom, sundress, cup, dye, isle, jacquard, shoulder, turtleneck, check, center, seam, jersey, athletic, dobby, strapless, pleat, utility, fleece, sweatshirt, pinafore, swim, gingham, wedge, cashmere, rib, lounge, georgette, control, tights, body, herringbone, line, espadrille, waistband, sock, metallic, minidress, board, boucl, reverse, weave, tech, joggers, split, cardigan, french, terry, knee, slit, poncho, trim, con, star, moon, inset, bib, space, chain, vintage, cutout, trench, shaker, stitch, twill, flat, trousers, trumpet, derby, peplum, illusion, mesh, bodysuit, romper, bandeau, keyhole, balloon, ribbed, cozy, slippers, solid, pliss, drawstring, hybrid, cap, merino, racerback, chemise, quarter, matthew, mixed, mountain, fine, gauge, coyote, rainbow, roll, zebra, cuff, portrait, pump, wave, girl, honeycomb, snake, puffer, skin, double, face, organza, butterfly, sheer, army, tunic, prairie, gore, tex, texture, sleep, sweatpants, loafer,$\ldots$ \\
\bottomrule
\end{tabular}
\label{tab:attributes}
\end{table*}

\subsection{Evaluation Metrics Explained}
We provide more information about BLEU, METEOR, ROUGH-L, CIDEr and SPICE metrics.
BLEU roughly measures the fraction of N-grams that are in common between a generated one and a groundtruth.
METEOR measures unigram precision and recall, extending the exact word matches to include similar words based on WordNet synonyms and stemmed tokens.
ROUGH-L counts the  number of  overlapping word sequences between the generated sentence and the groundtruth caption.
CIDEr measures the similarity of a generated sentence against a groundtrue caption using sentence similarity.
SPICE compares semantic propositional content between a generated sentence and a groundtruth.
