# Supplementary material for: Exploring External Knowledge for Accurate modeling of Visual and Language Problems
Source: arXiv:2302.08901 source file (2023-01-27)
Supplement: Supplementary file 2 [file 67_appendix.tex]

%\section{Appendices}

% \todo[inline,color=blue]{SK: Submission guidelines as comment. Supplementary material is possible but should not be part of the main paper and it is not guaranteed reviewers would check it.}

%\subsection{Datasets}
\section{Datasets}
We use two datasets GoodNews \cite{Biten_2019_CVPR} and NYTimes800k \cite{Tran2020Tell}.
Both datasets are collected by using The New York Times public API\footnote{https://developer.nytimes.com/apis}
For GoodNews dataset, since only the articles, captions, and
image URLs are publicly released, the images need to be
downloaded from the original source. 
Out of the 466K image URLs provided by \citet{Biten_2019_CVPR}, we were able to download 463K images, the remaining are broken links.
We use the same train, validation and test splits provided as \citet{Biten_2019_CVPR}. There are $421$K training, $18$K validation, and $23$K test captions.

NYTimes800k dataset is $70\%$ larger and more complete dataset of New York Times articles, images, and captions. 
The number of train, validation and test sets are $763$K, $8$K and $22$K respectively.
%$763217$, $7777$ and $21977$ separately.
Tab.~\ref{tab:dataset} presents a detailed comparison between GoodNews and NYTimes800k in terms of articles and captions length, and captions composition.

\begin{table}[t]
\small
    \centering
    \begin{tabular}{ccc}
    \toprule
    & GoodNews & NYTimes800k \\\midrule
    \# of articles & 257033 & 444914 \\
    \# of images & 462642 & 792971 \\
    Average article length & 653 & 892 \\
    Average caption length & 18 & 18 \\\hline
    \% of caption words that are & & \\
    nouns & 16\% & 16\% \\
    pronouns & 1\% & 1\% \\
    proper nouns & 23\% & 22\% \\
    verbs & 9\% & 9\% \\
    adjectives & 4\% & 4\% \\
    named entities & 27\% & 26\% \\ \hline
    \% of captions with & & \\
    named entities & 97\% & 96\% \\
    people’s names & 68\% & 68\% \\
    \bottomrule
    \end{tabular}
    \caption{Summary of news captioning datasets.}
    \label{tab:dataset}
\end{table}

\begin{table}[t]
    \centering
    \small
    \begin{tabular}{cccccc}
    \toprule
      Dataset & average len  & \% $> 512$ & \% $> 1000$  \\
      \midrule
      \good & 653  & 49.7\% & 18.2\% \\
      \nyt & 892  & 54.85\% & 21.92\% \\
      \bottomrule
    \end{tabular}
    \caption{Article length statistics for the \good and \nyt dataset.}
    \label{tab:len_stat}
    \vspace{-0.5cm}
\end{table}

We also show the article length statistics in Tab.~\ref{tab:len_stat}.
With approximate $50\%$ of the training articles having more than 512 tokens, MSTR technique is necessary to deal with this problem.

%\subsection{Template statistics}
\section{Template statistics and prediction results}

\begin{table*}[t]
    \centering
    \small
    \begin{adjustbox}{max width=\textwidth}
    \begin{tabular}{ccccccccccccccccc}
    \toprule
       template  & 1 & 2 & 3 & 4 & 5 & 6 & 7 & 8 & 9 & 10 & 11 & 12 & 13 & 14 & 15 & avg \\\midrule
        \% & 15.2 & 4.4 & 4.2 & 3.5 & 2.8 & 2.6 & 13.1 & 12.7 & 7.7 & 7.3 & 6.8 & 5.3 & 5.1 & 2.4 & 2.2 & -- \\
        who & $\times$ & $\times$ & $\times$ & $\times$ & $\times$ & $\times$ & $\times$ & $\times$ & $\times$ & $\times$ & $\times$ & $\times$ & $\times$ & -- & -- & -- \\
        when & $\times$ & -- & -- & $\times$ & -- & $\times$ & -- & -- & $\times$ & -- & $\times$ & -- & $\times$ & -- & -- & -- \\
        where & $\times$ & -- & $\times$ & $\times$ & -- & -- & -- & $\times$ & -- & -- & $\times$ & $\times$ & -- & $\times$ & -- & -- \\
        misc & $\times$ & -- & -- & -- & $\times$ & -- & -- & -- & -- & $\times$ & $\times$ & $\times$ & $\times$ & -- & -- & -- \\
        context & -- & -- & -- & -- & -- & -- & $\times$ & $\times$ & $\times$ & $\times$ & $\times$ & $\times$ & $\times$ & $\times$ & $\times$ & -- 
    \end{tabular}
    \end{adjustbox}
    \caption{Template class definition and its relation with different components. Note there are in total $2^5$ template class but we show the ones with over $2\%$ of samples which accounts for $96.2\%$ of the training data.}
    \label{tab:template_stat}
         \vspace{-0.3cm}
\end{table*}

\begin{table*}[t]
\small
	\centering
	\begin{adjustbox}{max width=\textwidth}
	\begin{tabular}{cc|cccccccccccc}
		%\toprule
		\cmidrule{3-14}
% 		 &
% 		 & \multirow{2}{*}{\textbf{\small{BLEU-4}}}
% 		 & \multirow{2}{*}{\textbf{\small{ROUGE}}}
% 		 & \multirow{2}{*}{\textbf{\small{METEOR}}}
% 		 & \multirow{2}{*}{\textbf{\small{CIDEr}}}
         & &
% 		 \multicolumn{2}{c}{\textbf{\small{Template Components}}}\\
        \multicolumn{2}{c}{\textbf{\small{Average}}} & \multicolumn{2}{c}{\textbf{\small{who}}} & \multicolumn{2}{c}{\textbf{\small{when}}} & \multicolumn{2}{c}{\textbf{\small{where}}} & \multicolumn{2}{c}{\textbf{\small{misc}}} & \multicolumn{2}{c}{\textbf{\small{context}}} \\
		 \cmidrule{3-14}
		  & & \small{$\overline{P}$} & \small{$\overline{R}$}  & P & R & P & R & P & R & P & R & P & R  \\
		\midrule
		%\multirow{12}{*}{\rotatebox[origin=c]{90}{GoodNews}}
		\multirow{6}{*}[-1cm]{\rotatebox[origin=c]{90}{\good}}
		%& VGG+LSTM \cite{Ramisa18} & 0.31 & 6.38 & 1.66 & 1.28 & -- & -- & -- & -- \\\cmidrule{2-10}
		
		& Tell~\cite{Tran2020Tell} & 69.52 & 63.31 & 90.44 & 83.48 & 59.25 & 58.78 & 62.90 & 66.67 & 51.59 & 42.50 & 83.43 & 65.13 \\
		& Tell (full)~\cite{Tran2020Tell} & 71.55 & 64.93 & 91.49 & 85.89 & 63.04 & 60.69 & 65.45 & 66.90 & 53.27 & 46.00 & 84.50 & 65.19 \\
		 \cmidrule{2-14}
		 %&  Longformer & 5.62 & 20.37 & 9.88 & 48.01 & 22.05 & 16.05 \\
		 & \name (zero-out text) &  18.92 & 16.77 & 23.15 & 21.28 & 16.96 & 15.12 & 18.63 & 17.86 & 13.14 & 11.58 & 22.72 & 18.01 \\
		 & \name (zero-out image) & 48.74 & 46.29 & 63.09 & 60.21 & 39.82 & 37.40 & 44.96 & 42.60 & 25.50 & 23.03 & 70.33 & 68.21 \\
		 & \name (image only) &  19.07 & 17.13 & 23.38 & 21.61 & 17.15 & 15.52 & 18.70 & 17.92 & 13.31 & 11.72 & 22.81 & 18.88 \\
		 & \name (text only) & 49.56 & 46.98 & 63.89 & 60.89 & 40.73 & 38.11 & 45.81 & 43.25 & 26.20 & 23.73 & 71.17 & 68.92 \\
		 & \name (Longformer) & 74.07 & 58.86 & 94.46 & 87.45 & 63.29 & 26.66 & 71.45 & 62.66 & 54.67 & 45.30 & 86.46 & 72.25 \\
		 & \name (auto) & 75.51 & 66.27 & 94.77 & 86.59 & 66.15 & 64.19 & 71.21 & 67.79 & \textbf{58.92} & 46.12 & 86.52 & 66.65 \\
		 &  \namens+\neeshort (auto) & 74.42 & 68.53 & 94.64 & 88.65 & 64.66 & 64.26 & 70.54 & 68.22 & 55.93 & 48.65 & 86.34 & 72.88 \\
		 & \namens+MSTR (auto) & 75.57 & \textbf{70.04} & 94.32 & \textbf{91.00} & \textbf{68.75} & \textbf{66.91} & 71.50 & \textbf{70.16} & 56.81 & \textbf{49.07} & 86.49 & \textbf{73.07} \\
		 & \namens+MSTR+\neeshort (auto) &  \textbf{75.83} & 
		 68.85 & \textbf{95.75} & 90.01 & 66.72 & 64.45 & \textbf{72.19} & 69.38 & 57.33 & 48.48 & \textbf{87.19} & 71.96 \\
		 \cmidrule{2-14}
		 & \name (oracle) &  \textit{92.69} & \textit{87.86} & \textit{95.07} & \textit{88.21} & \textit{97.09} & \textit{95.10} & \textit{88.50} & \textit{84.02} & \textit{84.07} & \textit{78.01} & \textit{98.75} & \textit{93.97} \\
		 & \namens+MSTR+\neeshort (oracle) &  \textit{92.46} & \textit{87.55} & \textit{95.07} & \textit{88.79} & \textit{97.00} & \textit{93.86} & \textit{88.09} & \textit{83.79} & \textit{83.43} & \textit{75.81} & \textit{98.70} & \textit{95.50}  \\
		\midrule
		\midrule
		\multirow{6}{*}[-0.5cm]{\rotatebox[origin=c]{90}{\nyt}}
		 & Tell~\cite{Tran2020Tell} & 67.13 & 62.24 & 86.44 & 79.65 & 57.45 & 63.93 & 61.08 & 72.19 & 46.30 & 36.99 & 84.39 & 58.44 \\
		 & Tell (full)~\cite{Tran2020Tell} & 69.72 & 63.52 & 88.91 & 82.92 & 61.30 & 65.83 & 63.97 & 73.52 & 49.40 & 39.34 & 85.07 & 56.01 \\
		 \cmidrule{2-14}
		 %&  Longformer & 5.65 & 19.84 & 9.83 & 42.72 & 23.67 & 18.55 \\
		 & \name (zero-out text) & 18.87 & 16.53 & 22.96 & 20.96 & 16.52 & 14.88 & 18.01 & 17.21 & 13.02 & 11.34 & 23.84 & 18.26 \\
		 & \name (zero-out image) & 53.71 & 51.29 & 79.74 & 68.10 & 41.83 & 45.91 & 51.07 & 48.82 & 26.89 & 30.19 & 69.02 & 63.43 \\
		 & \name (image only) & 19.40 & 17.12 & 23.51 & 21.55 & 16.98 & 15.51 & 18.54 & 17.69 & 13.61 & 11.82 & 24.36 & 19.03 \\
		 & \name (text only) & 54.89 & 52.31 & 80.96 & 69.08 & 44.02 & 47.02 & 52.39 & 49.75 & 28.15 & 31.23 & 68.93 & 64.47 \\
		 & \name (Longformer) & 68.93 & 56.67 & 88.24 & 83.72 & 60.59 & 28.63 & 65.10 & 65.73 & 46.64 & 38.87 & 84.08 & 66.40 \\
		 & \name (auto) & 73.37 & 65.79 & 92.89 & 85.61 & \textbf{64.62} & \textbf{66.90} & 69.69 & 72.22 & \textbf{53.25} & 41.53 & 86.38 & 62.69 \\
		 &  \namens+\neeshort (auto) & 73.02 & \textbf{66.54} & \textbf{93.54} & \textbf{86.45} & 63.54 & 64.44 & 68.43 & \textbf{74.59} & 52.81 & \textbf{44.37} & 86.80 & 62.86 \\
		 &  \namens+MSTR (auto) & 73.36 & 66.30 & 93.21 & 85.97 & 64.59 & 66.60 & 70.32 & 73.25 & 51.67 & 42.62 & 87.02 & \textbf{63.08} \\
		 & \namens+MSTR+\neeshort (auto) &  \textbf{73.51} & 65.49 & 93.10 & 86.44 & 64.09 & 65.05 & \textbf{70.40} & 74.26 & 52.82 & 41.05 & \textbf{87.15} & 60.66 \\
		 \cmidrule{2-14}
		 & \name (oracle) & \textit{90.76} & \textit{87.99} & \textit{93.35} & \textit{87.63} & \textit{95.42} & \textit{94.04} & \textit{87.59} & \textit{86.57} & \textit{78.58} & \textit{76.08} & \textit{98.86} & \textit{95.65} \\
		 & \namens+MSTR+\neeshort (oracle) &  \textit{90.07} & \textit{87.92} & \textit{92.88} & \textit{88.16} & \textit{94.70} & \textit{93.59} & \textit{86.86} & \textit{87.28} & \textit{77.26} & \textit{75.03} & \textit{98.67} & \textit{95.55} \\
		\bottomrule
	\end{tabular}
	\end{adjustbox}
	\caption {Precision and Recall results of each template component prediction on \good and \nyt. We highlight the \textbf{best} model in bold.\label{tab:results}}
\end{table*}

We show the composition in terms of components and the percentage of the template classes of the whole GoodNews dataset in Tab.~\ref{tab:template_stat}.

We also report in Tab.~\ref{tab:results} detailed template components precision and recall scores for different variants of our model and the Tell baseline on the two datasets.

%\subsection{Training details}
\section{Implementation and Training details}

Following \citet{Tran2020Tell}, we set the hidden size of the input features $d_I=2048$, $d_T=1024$ and $d_E=300$ and the number of heads $H=16$.
We use the Adam optimizer~\cite{kingma2015} with $\beta_1=0.9$, $\beta_2=0.98$, $\epsilon=10^{-6}$.
The number of tokens in the vocabulary $K=50264$ and $d^{Wiki}=300$.
We use a maximum batch size of $16$ and training is stopped after the model has seen 6.6 million examples, corresponding to $16$ epochs on \good and $9$ epochs on \nyt. 
The components prediction head in Fig. 2 of the main chapter is a Linear layer followed by an output layer with hidden states dimension equal to $1024$.
The training pipeline is written in PyTorch~\cite{paszke2017automatic} using
the AllenNLP framework~\cite{gardner2018allennlp}. The RoBERTa model and
dynamic convolution code are adapted from fairseq~\cite{ott2019fairseq}.
Training is done with mixed precision to reduce the memory footprint and allow our full model to be trained on a single GPU.
The models take 4 to 6 days to train on one V-100 GPU on both datasets.

\section{Model Difference Between Tell and \name}

As shown in Tab.~\ref{tab:tell_vs_tgnc}, our model shares some components with the baseline model Tell~\cite{Tran2020Tell}.
\name and Tell both use an image and text encoder and a Transformer decoder.
However, \name applies template guidance to model the journalistic guidelines for caption generation.

\begin{table*}[t]
    \centering
    \small
    \begin{adjustbox}{max width=\textwidth}
    \begin{tabular}{cccccccccc}
    \toprule
         & image & text & template guidance & faces & objects  & weighted RoBERTa & location aware & decoder & \# of parameters \\\midrule
         Tell & $\times$ & $\times$  &  -- & -- & -- & -- & -- & Transformer & 125M\\
         Tell (full) & $\times$ & $\times$ &  -- & $\times$ & $\times$ & $\times$ & $\times$ & Transformer & 200M \\
         \name & $\times$ & $\times$  &  $\times$ & -- & -- & -- & -- & Transformer & 205M \\
         \bottomrule
    \end{tabular}
    \end{adjustbox}
    \caption{The difference between \name and Tell \cite{Tran2020Tell}. Tell can be regarded as a variant of \name without template guidance. $\times$: having this technique. --: not having this one.}
    \label{tab:tell_vs_tgnc}
\end{table*}

\section{Human evaluation}

We have conducted a human evaluation of 200 article-image pairs. Below the article and the image, we displayed either the ground truth caption or a caption generated by Tell or one of our model variant.
We ask the annotators to rate each caption as follows:
\begin{itemize}
    \item How well does the caption describe the IMAGE? Regardless of how fluent it is.
    \begin{itemize}
        \item 1 = Very bad (Does not describe the image)
        \item 2 = Somewhat bad (Describes the image, but contradictory to or missing key information from the image) 
        \item 3 = Somewhat good (Describes the image, no contradictions but missing key information from the image) 
        \item 4 = Very good (Describes the image, no contradictions and contains the key information from the image)
    \end{itemize}
    \item How well does the caption summarize the ARTICLE? Regardless of how fluent it is.
    \begin{itemize}
        \item 1 = Very bad (Not relevant to the topic)
        \item 2 = Somewhat bad (Covers the right topic, but contradicting the article or missing key facts)
        \item 3 = Somewhat good (Covers the right topic, no contradictions with the article, but missing key facts)
        \item 4 = Very good (Covers the right topic, no contradictions with the article, and contains the key facts)
    \end{itemize}
    \item How easy or hard is it to understand the SENTENCE? Regardless of how well it describes the image or article.
    \begin{itemize}
        \item 1 = Very hard or doesn’t make sense
        \item 2 = Somewhat hard
        \item 3 = Somewhat easy
        \item 4 = Very easy to understand
    \end{itemize}
\end{itemize}

\begin{figure}[t]
         \includegraphics[width=\columnwidth]{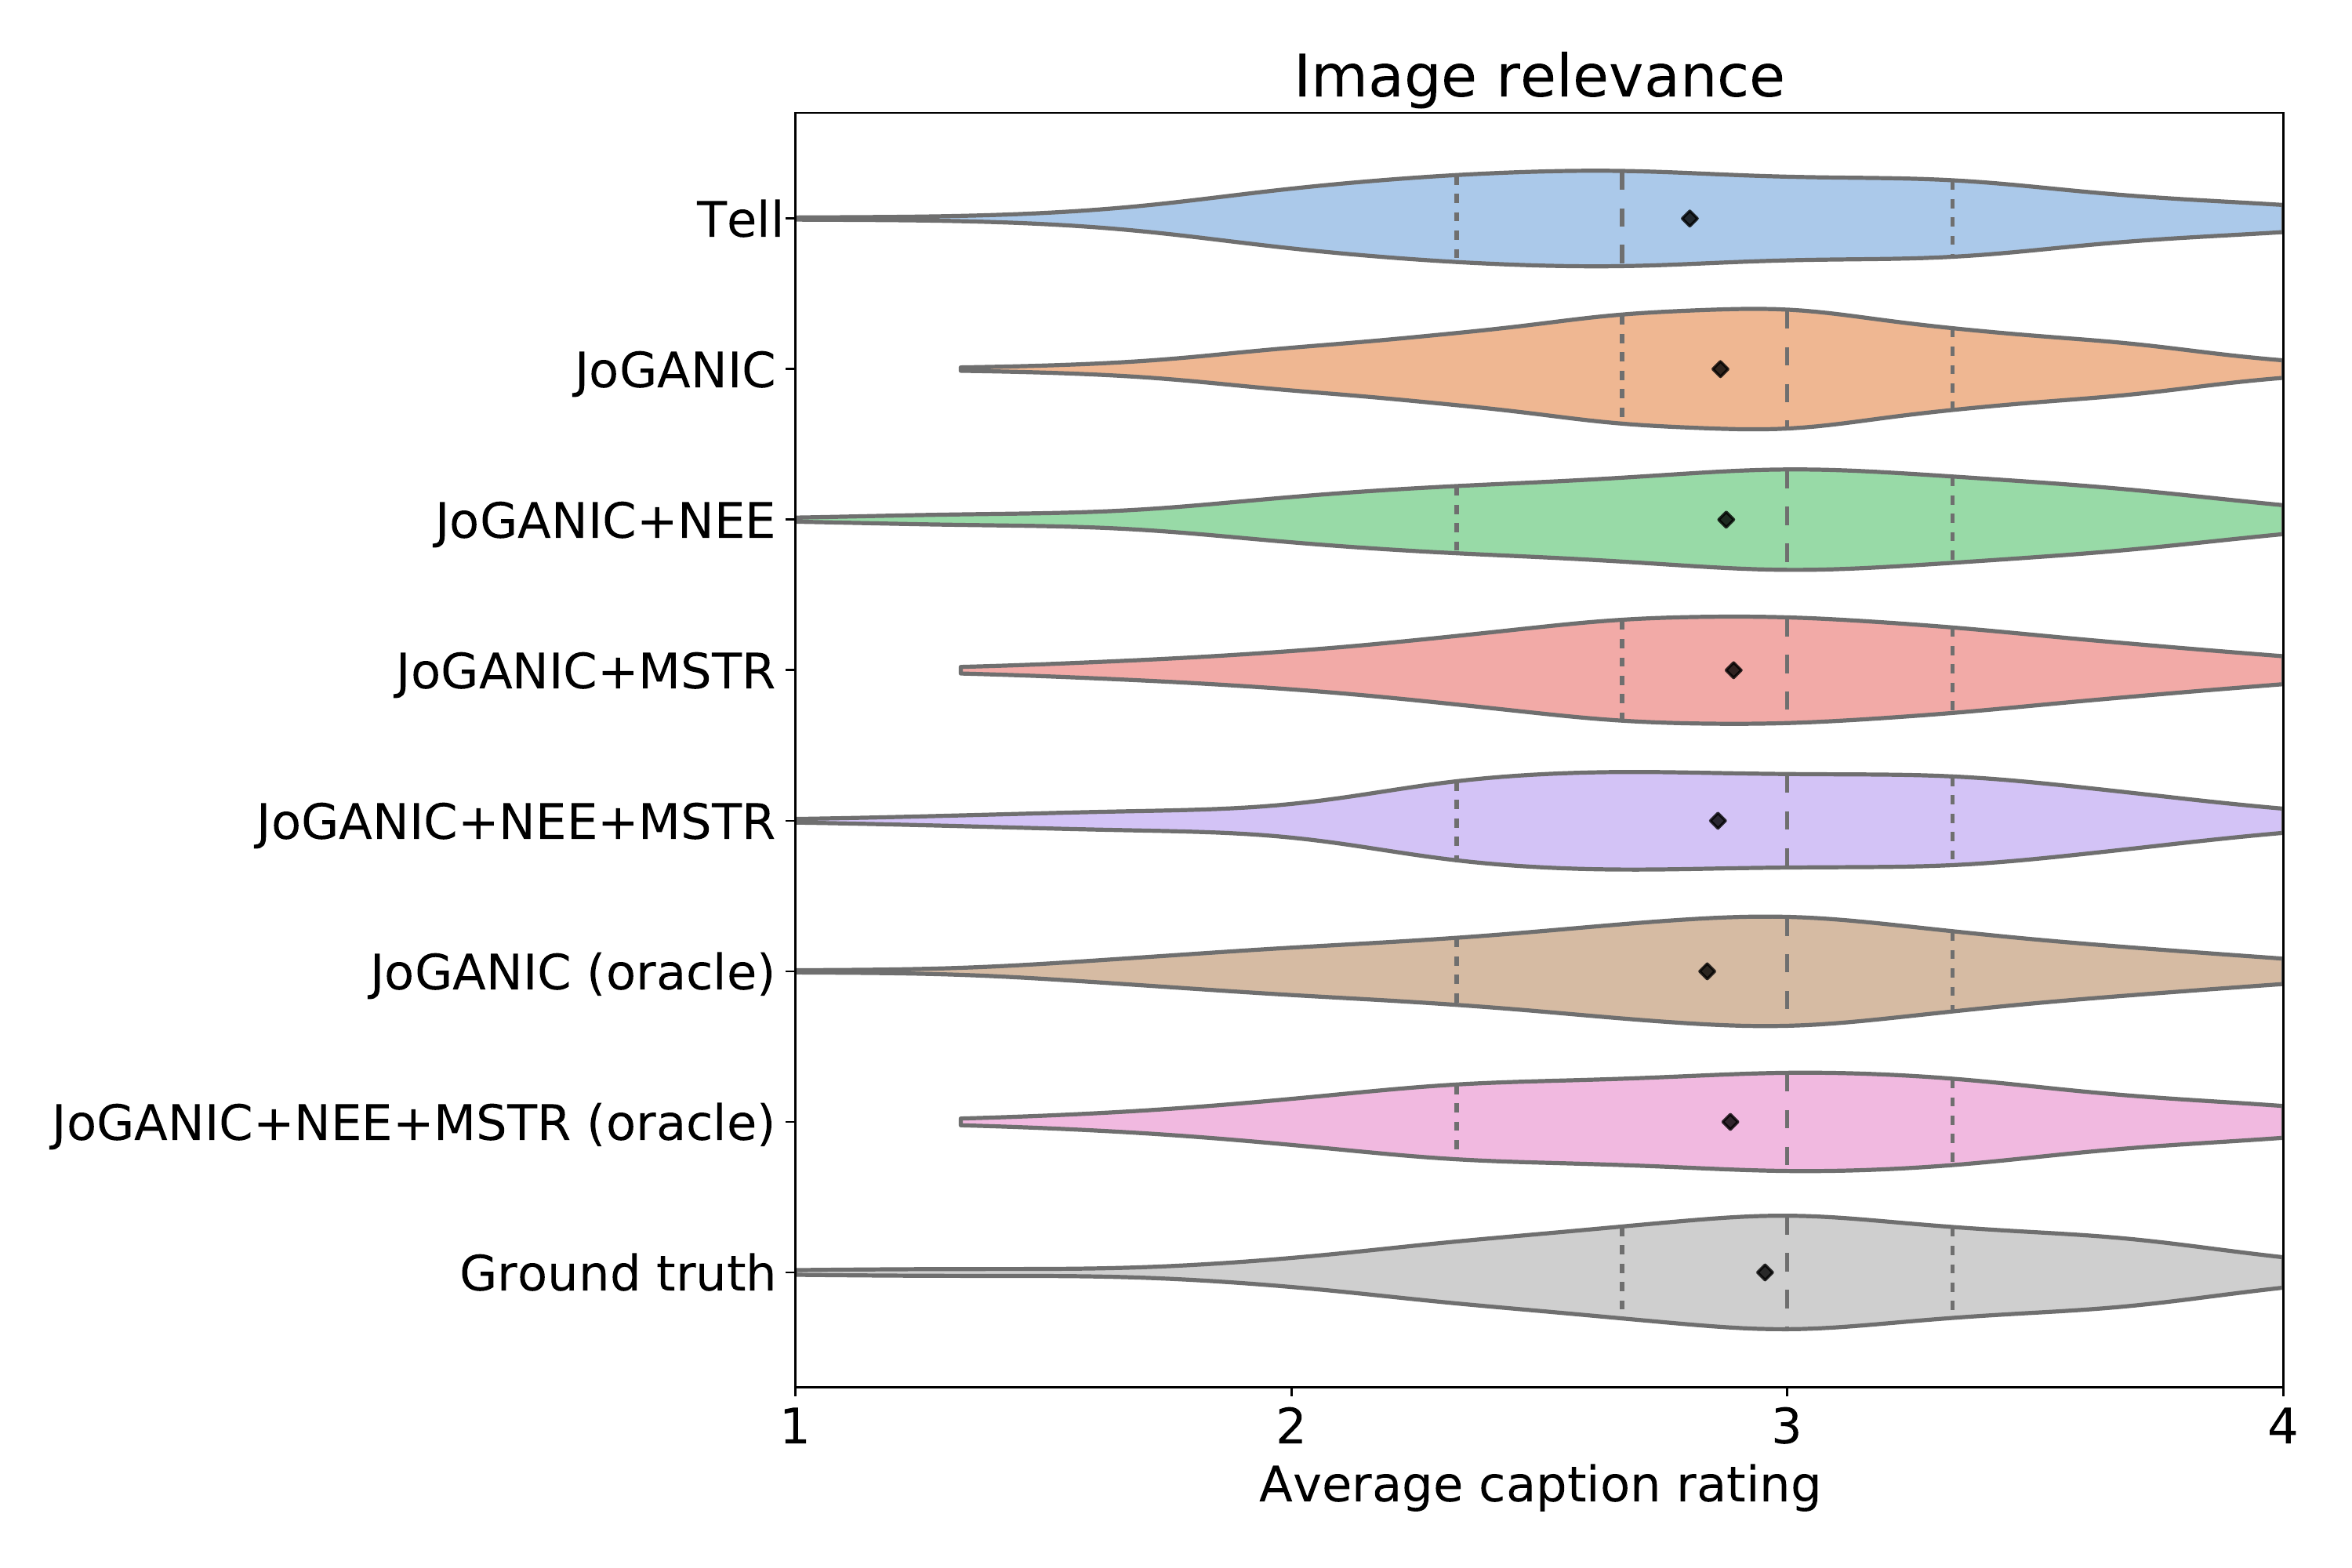}
         \caption{Image relevance ratings distributions.}
         \label{fig:humaneval_img}
         \vspace{-0.3cm}
\end{figure}

\begin{figure}[t]
         \includegraphics[width=\columnwidth]{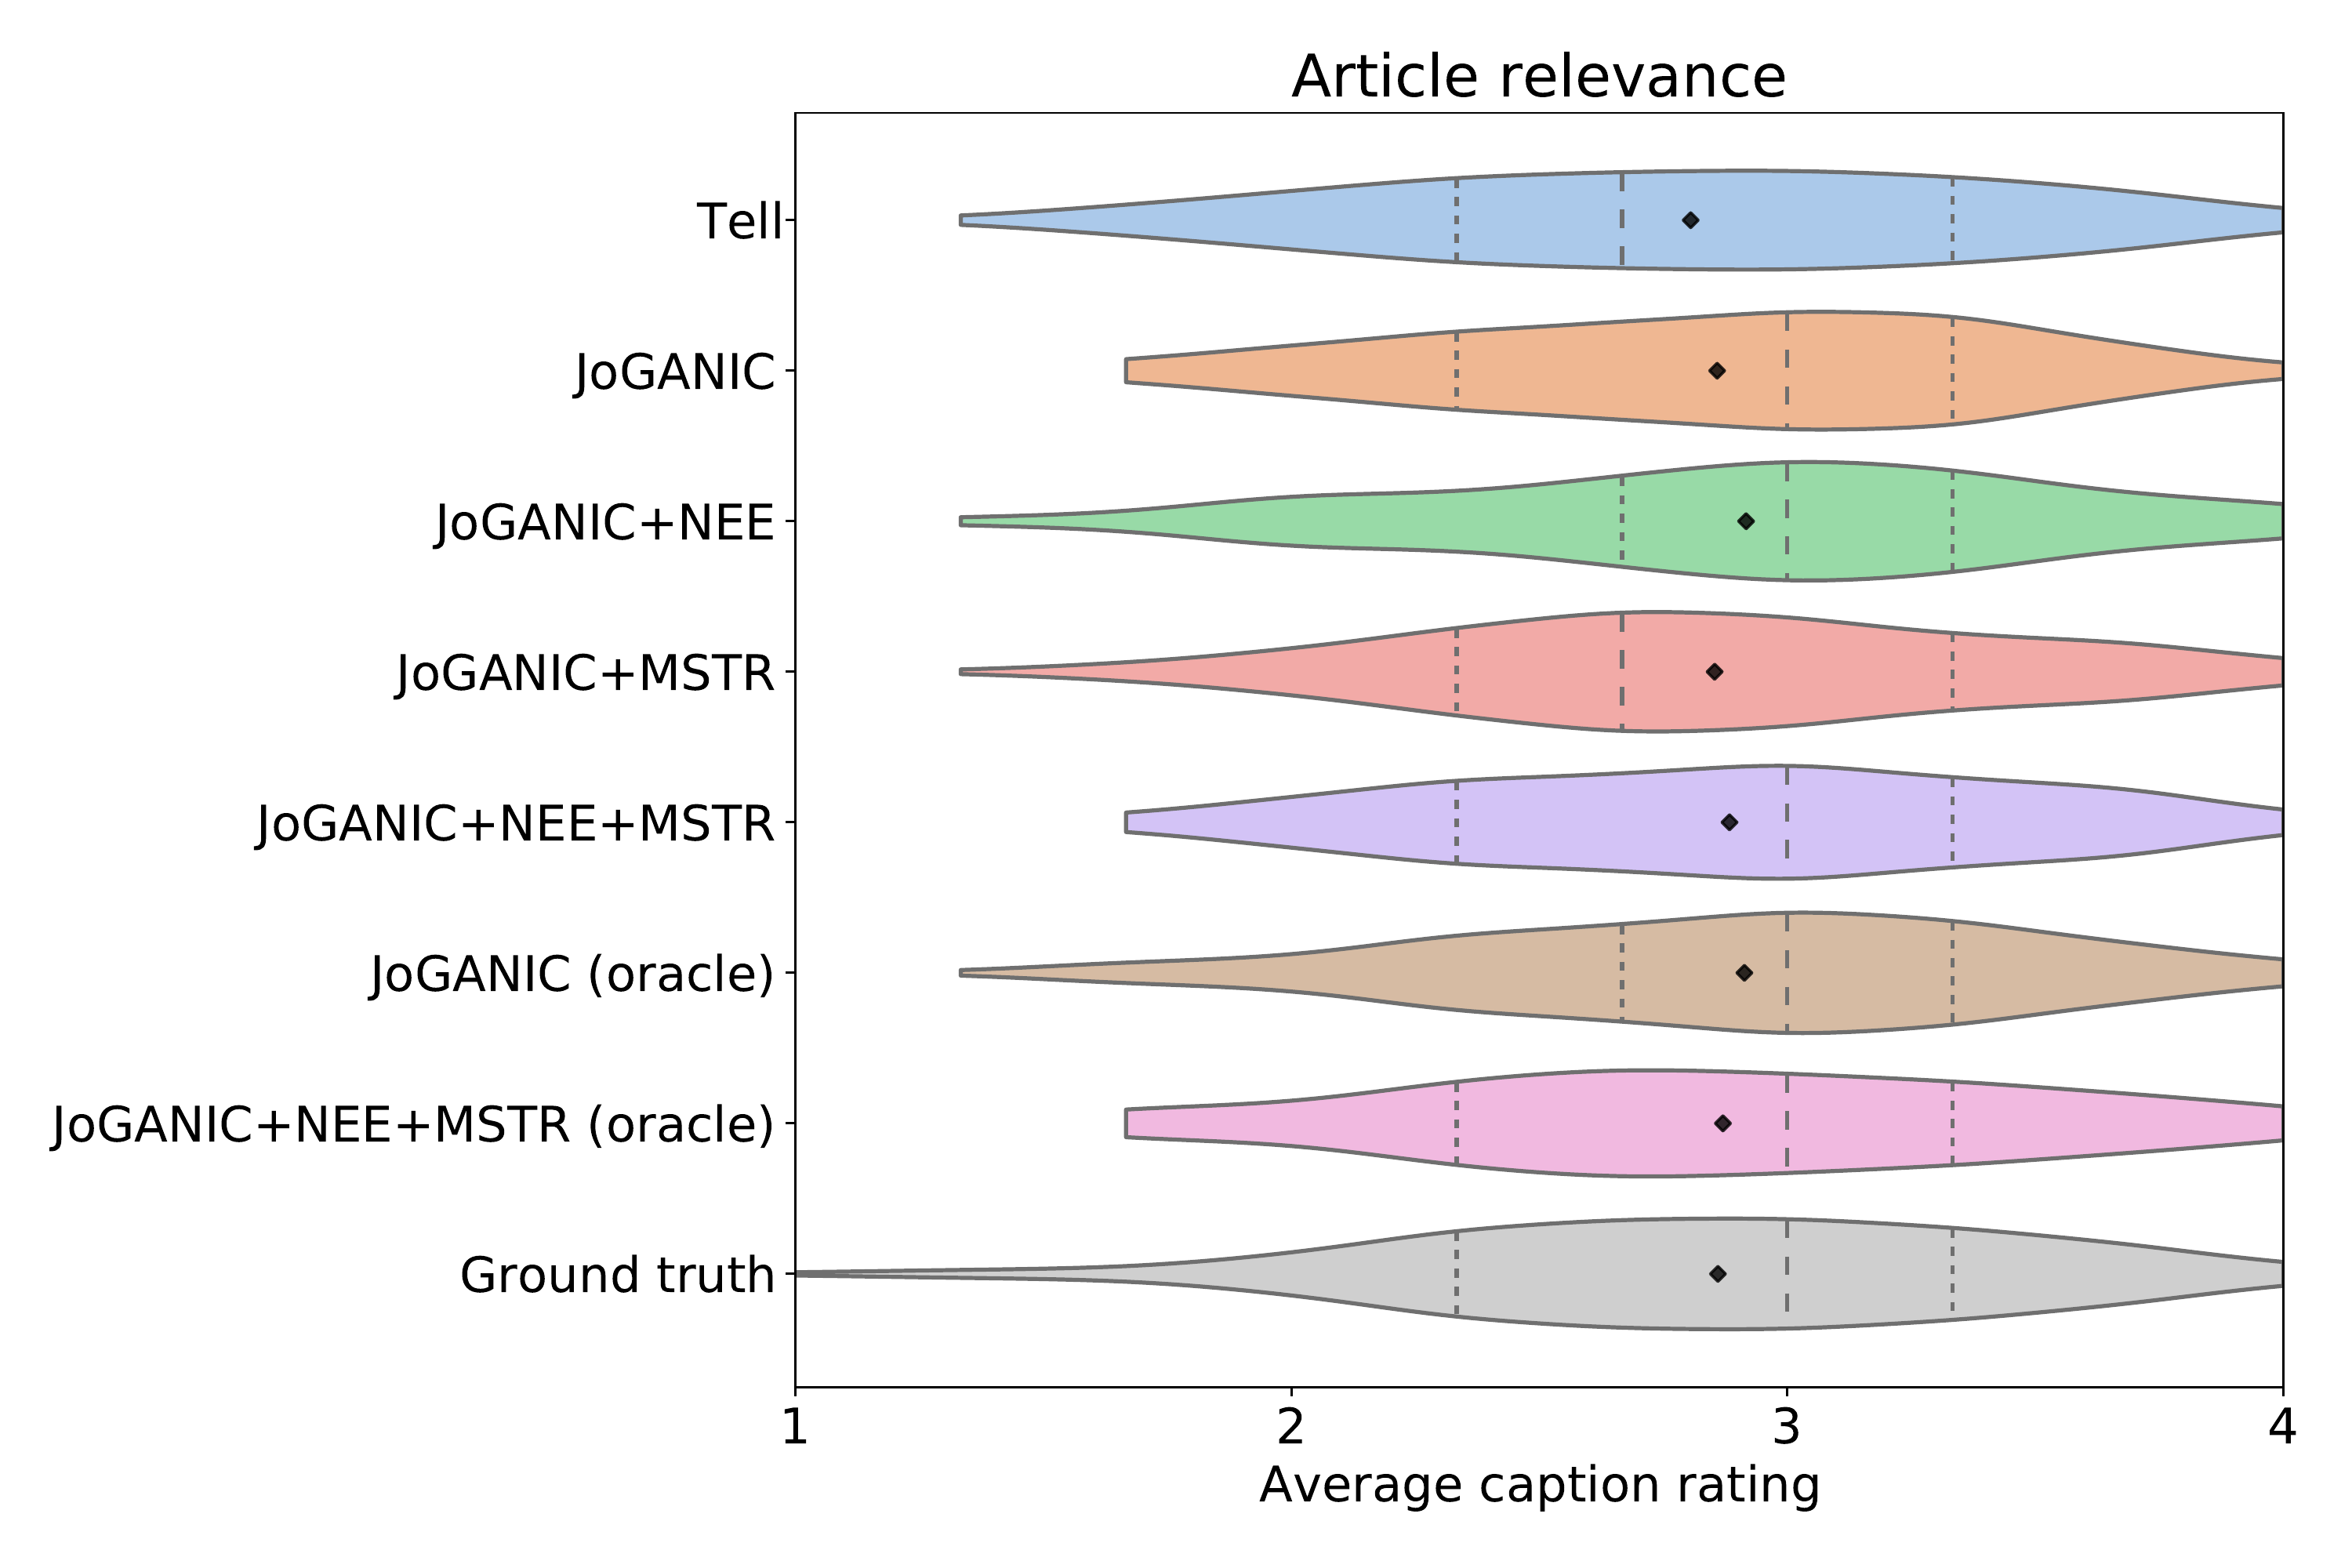}
         \caption{Article relevance ratings distributions.}
         \label{fig:humaneval_art}
         \vspace{-0.3cm}
\end{figure}
     
\begin{figure}[t]
         \includegraphics[width=\columnwidth]{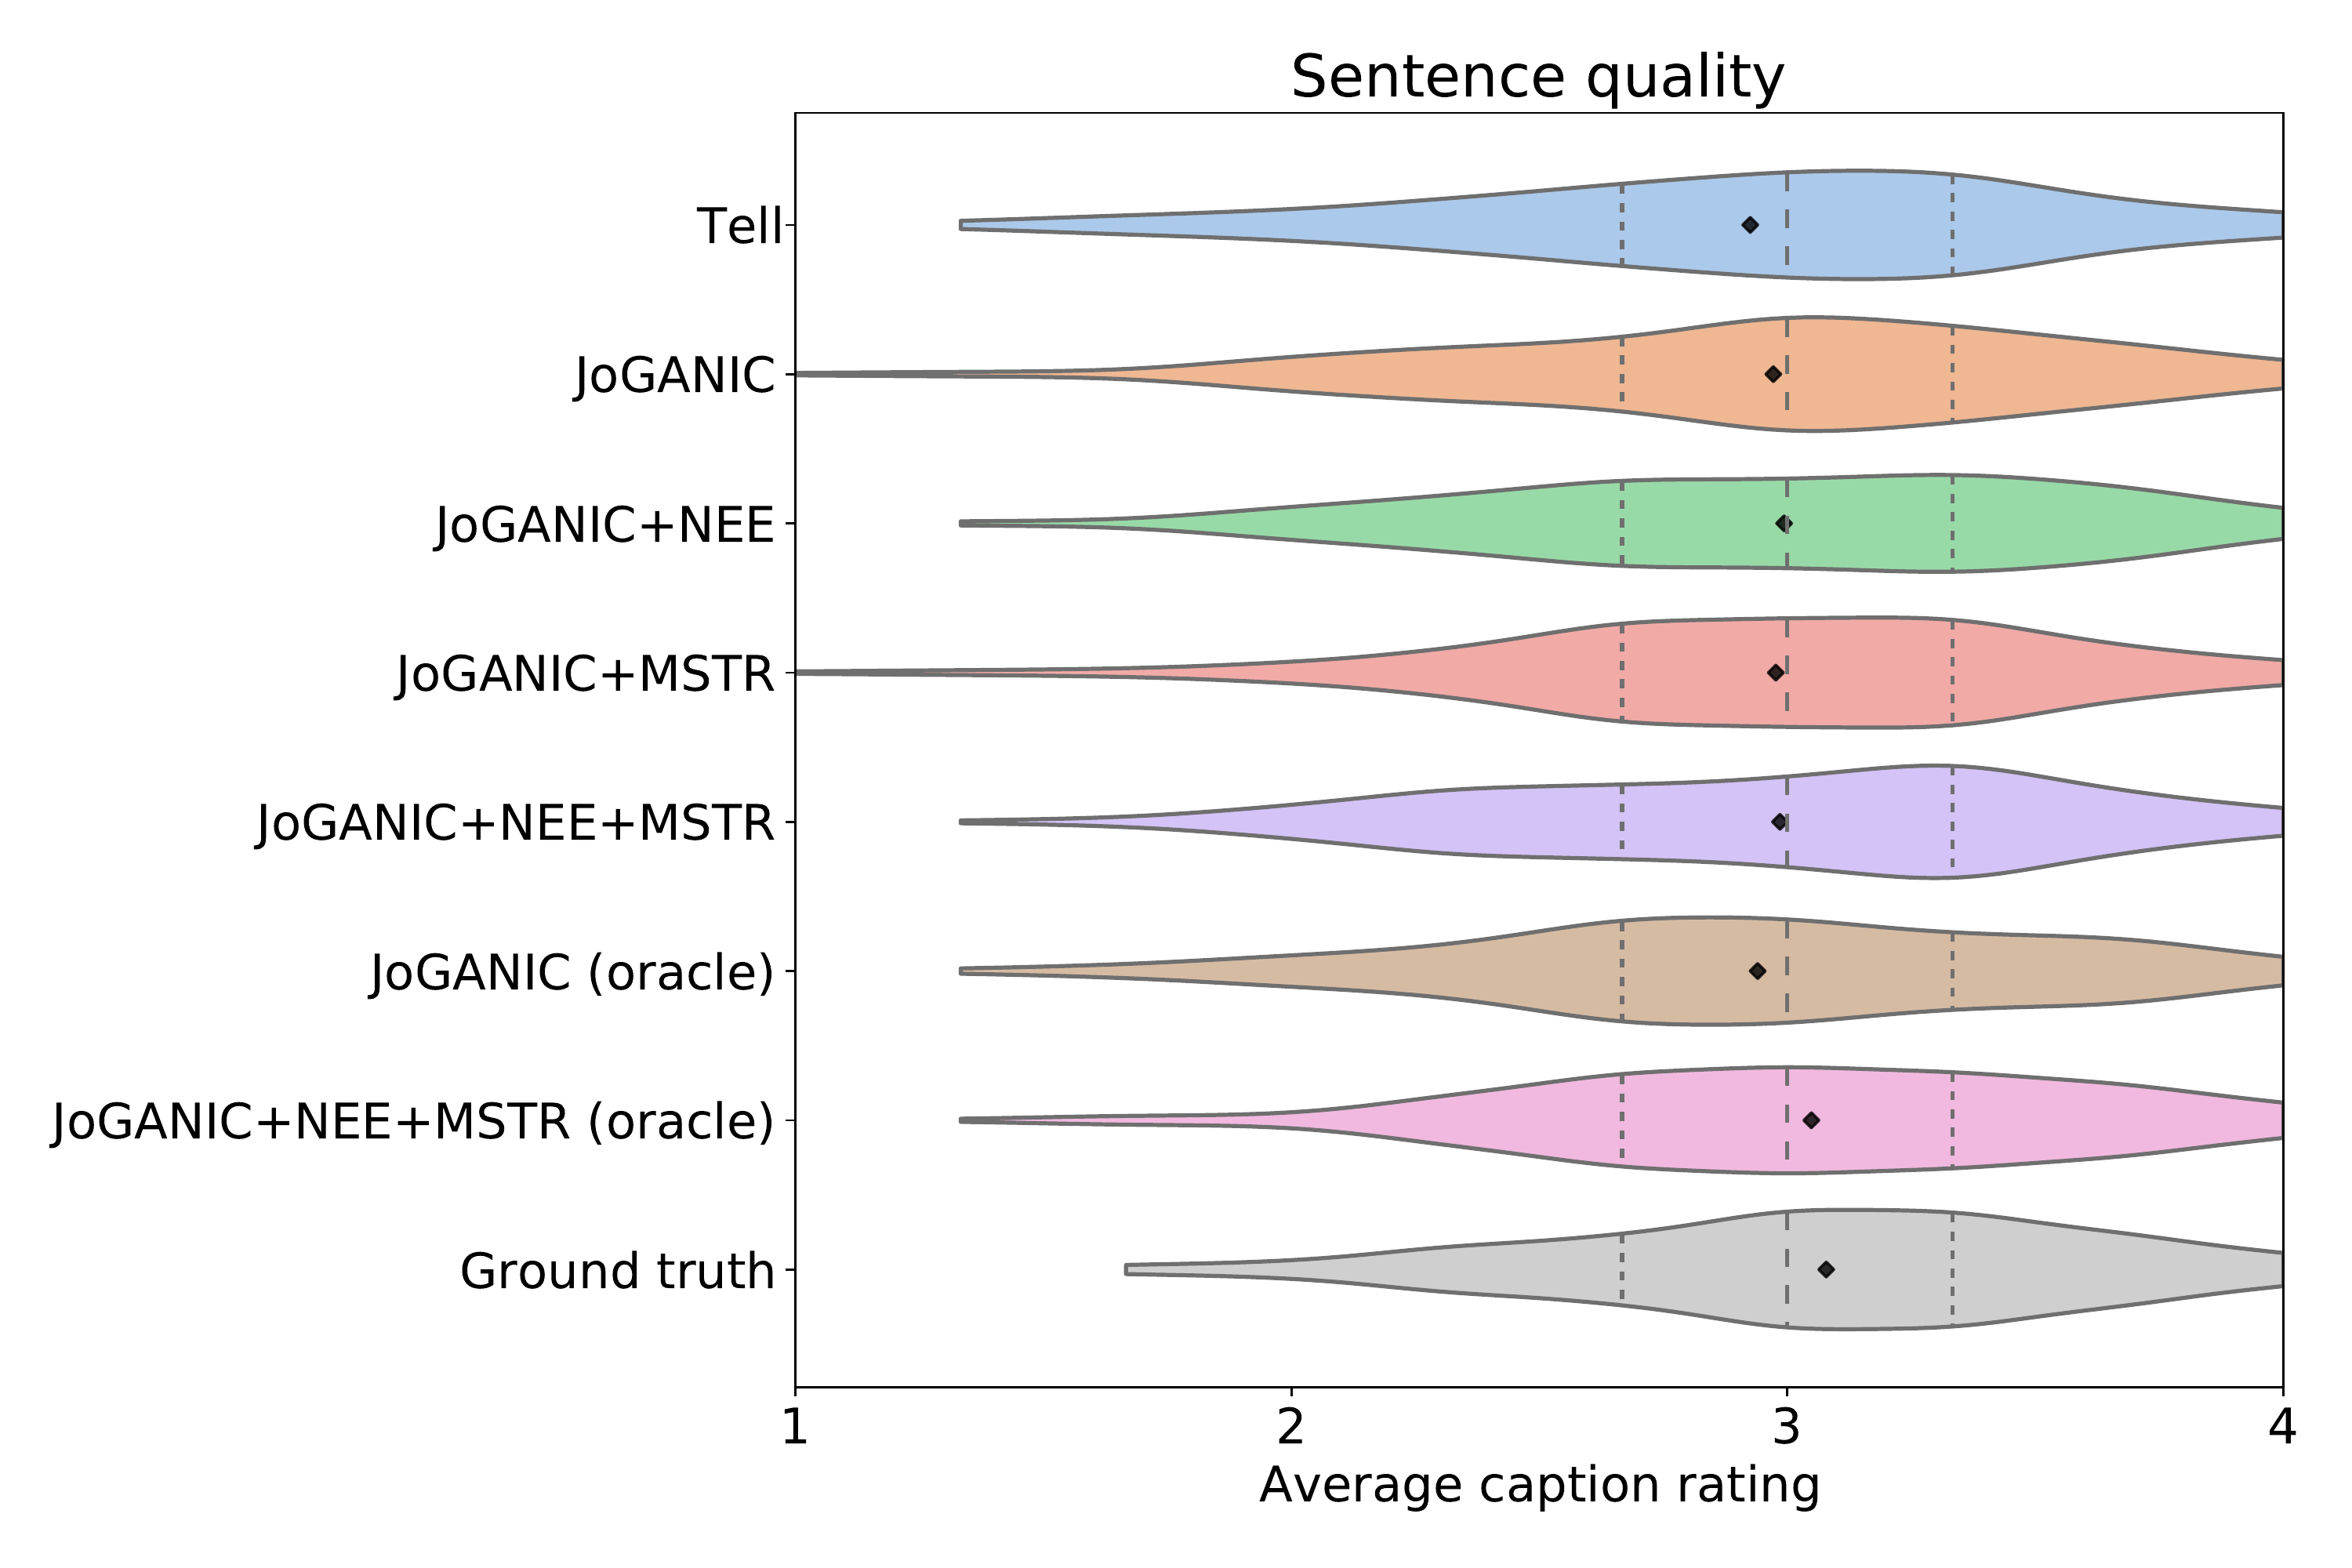}
         \caption{Sentence quality ratings distributions.}
         \label{fig:humaneval_sen}
         \vspace{-0.3cm}
\end{figure}

Each image-article pair is shown to three different annotators, thus each caption is rated three times. We average the rating for each caption, and then plot the image relevance, article relevance and sentence quality ratings statistics as violin plots in Figure~\ref{fig:humaneval_img}, Figure~\ref{fig:humaneval_art} and Figure~\ref{fig:humaneval_sen}, respectively. 
In each of these plots, the median is reported as a large dashed line, the first and third quartile as thinner dashed lines and the mean score as the black diamond.
The varying height of each violin represent the number of samples having the corresponding rating.
We can observe that all distributions are somewhat similar, but the Tell model is generally produces the lowest rated captions. The basic JoGANIC is a bit better, while more advanced variations of our model produce captions that are rated higher and really similarly to the ground truth captions.

% \begin{figure*}
%      \centering
%      \begin{subfigure}[b]{0.3\textwidth}
%          \centering
%          \includegraphics[width=\textwidth]{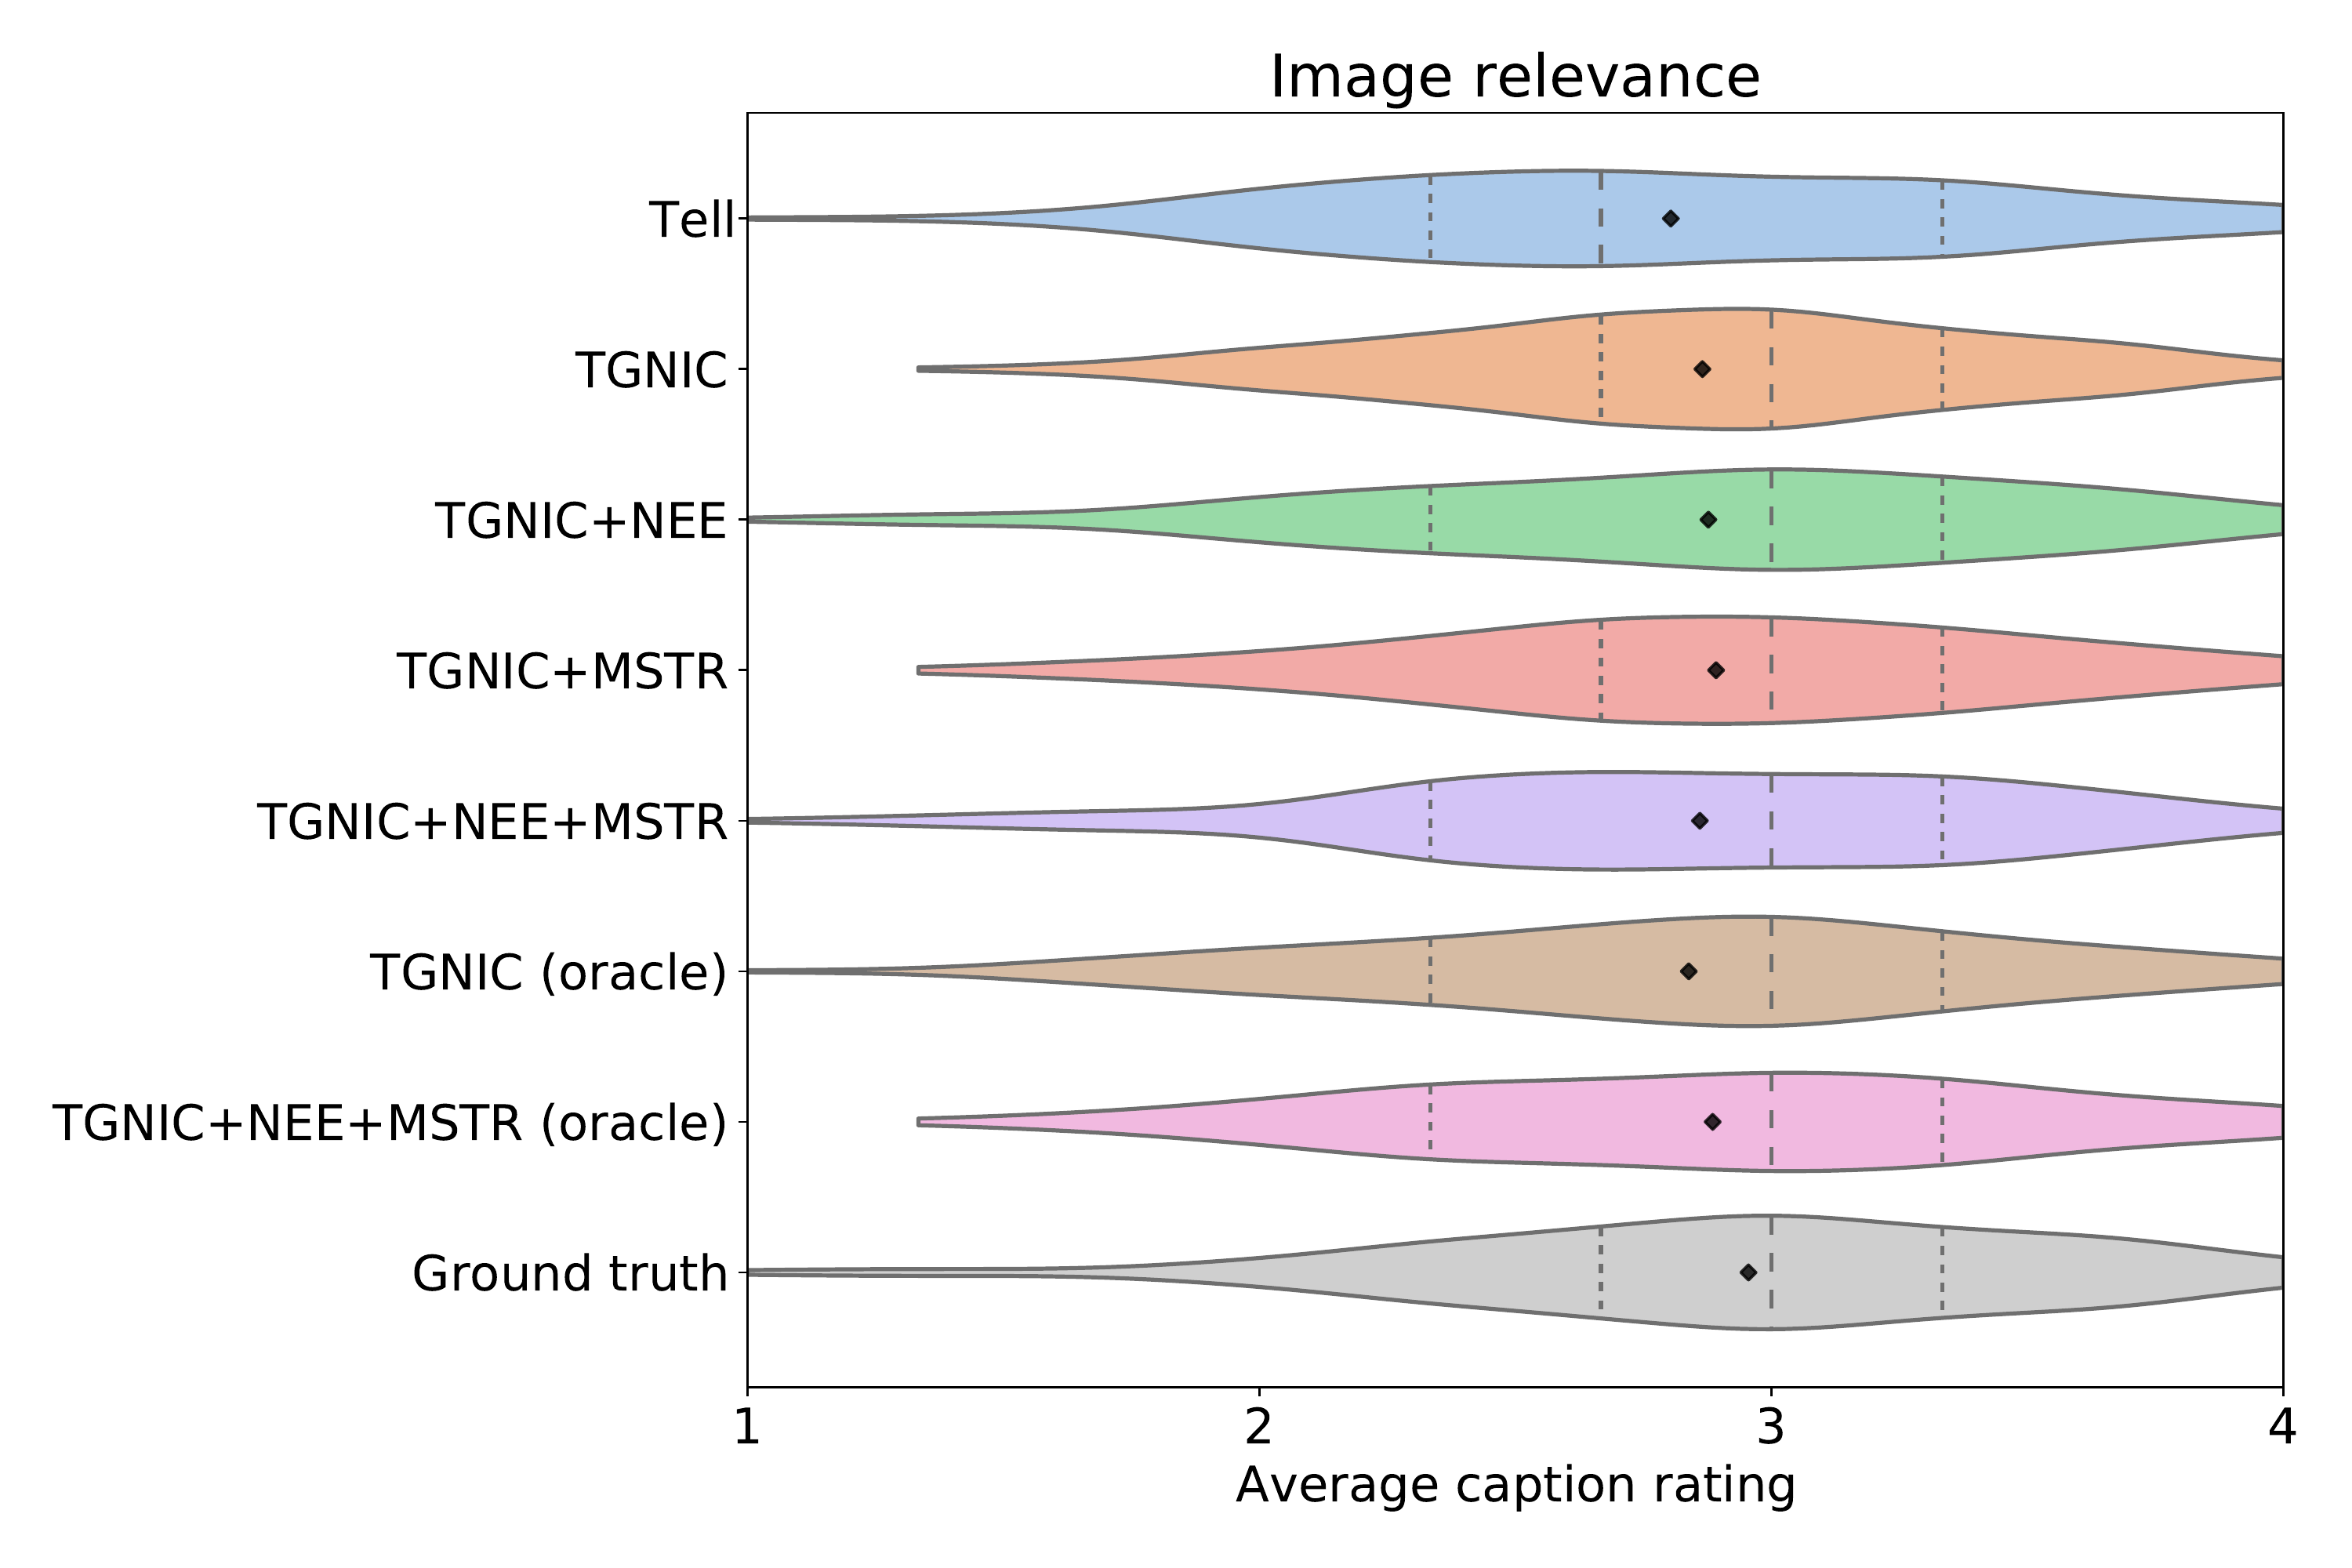}
%          \caption{Image relevance}
%          \label{fig:humaneval_img}
%      \end{subfigure}
%      \hfill
%      \begin{subfigure}[b]{0.3\textwidth}
%          \centering
%          \includegraphics[width=\textwidth]{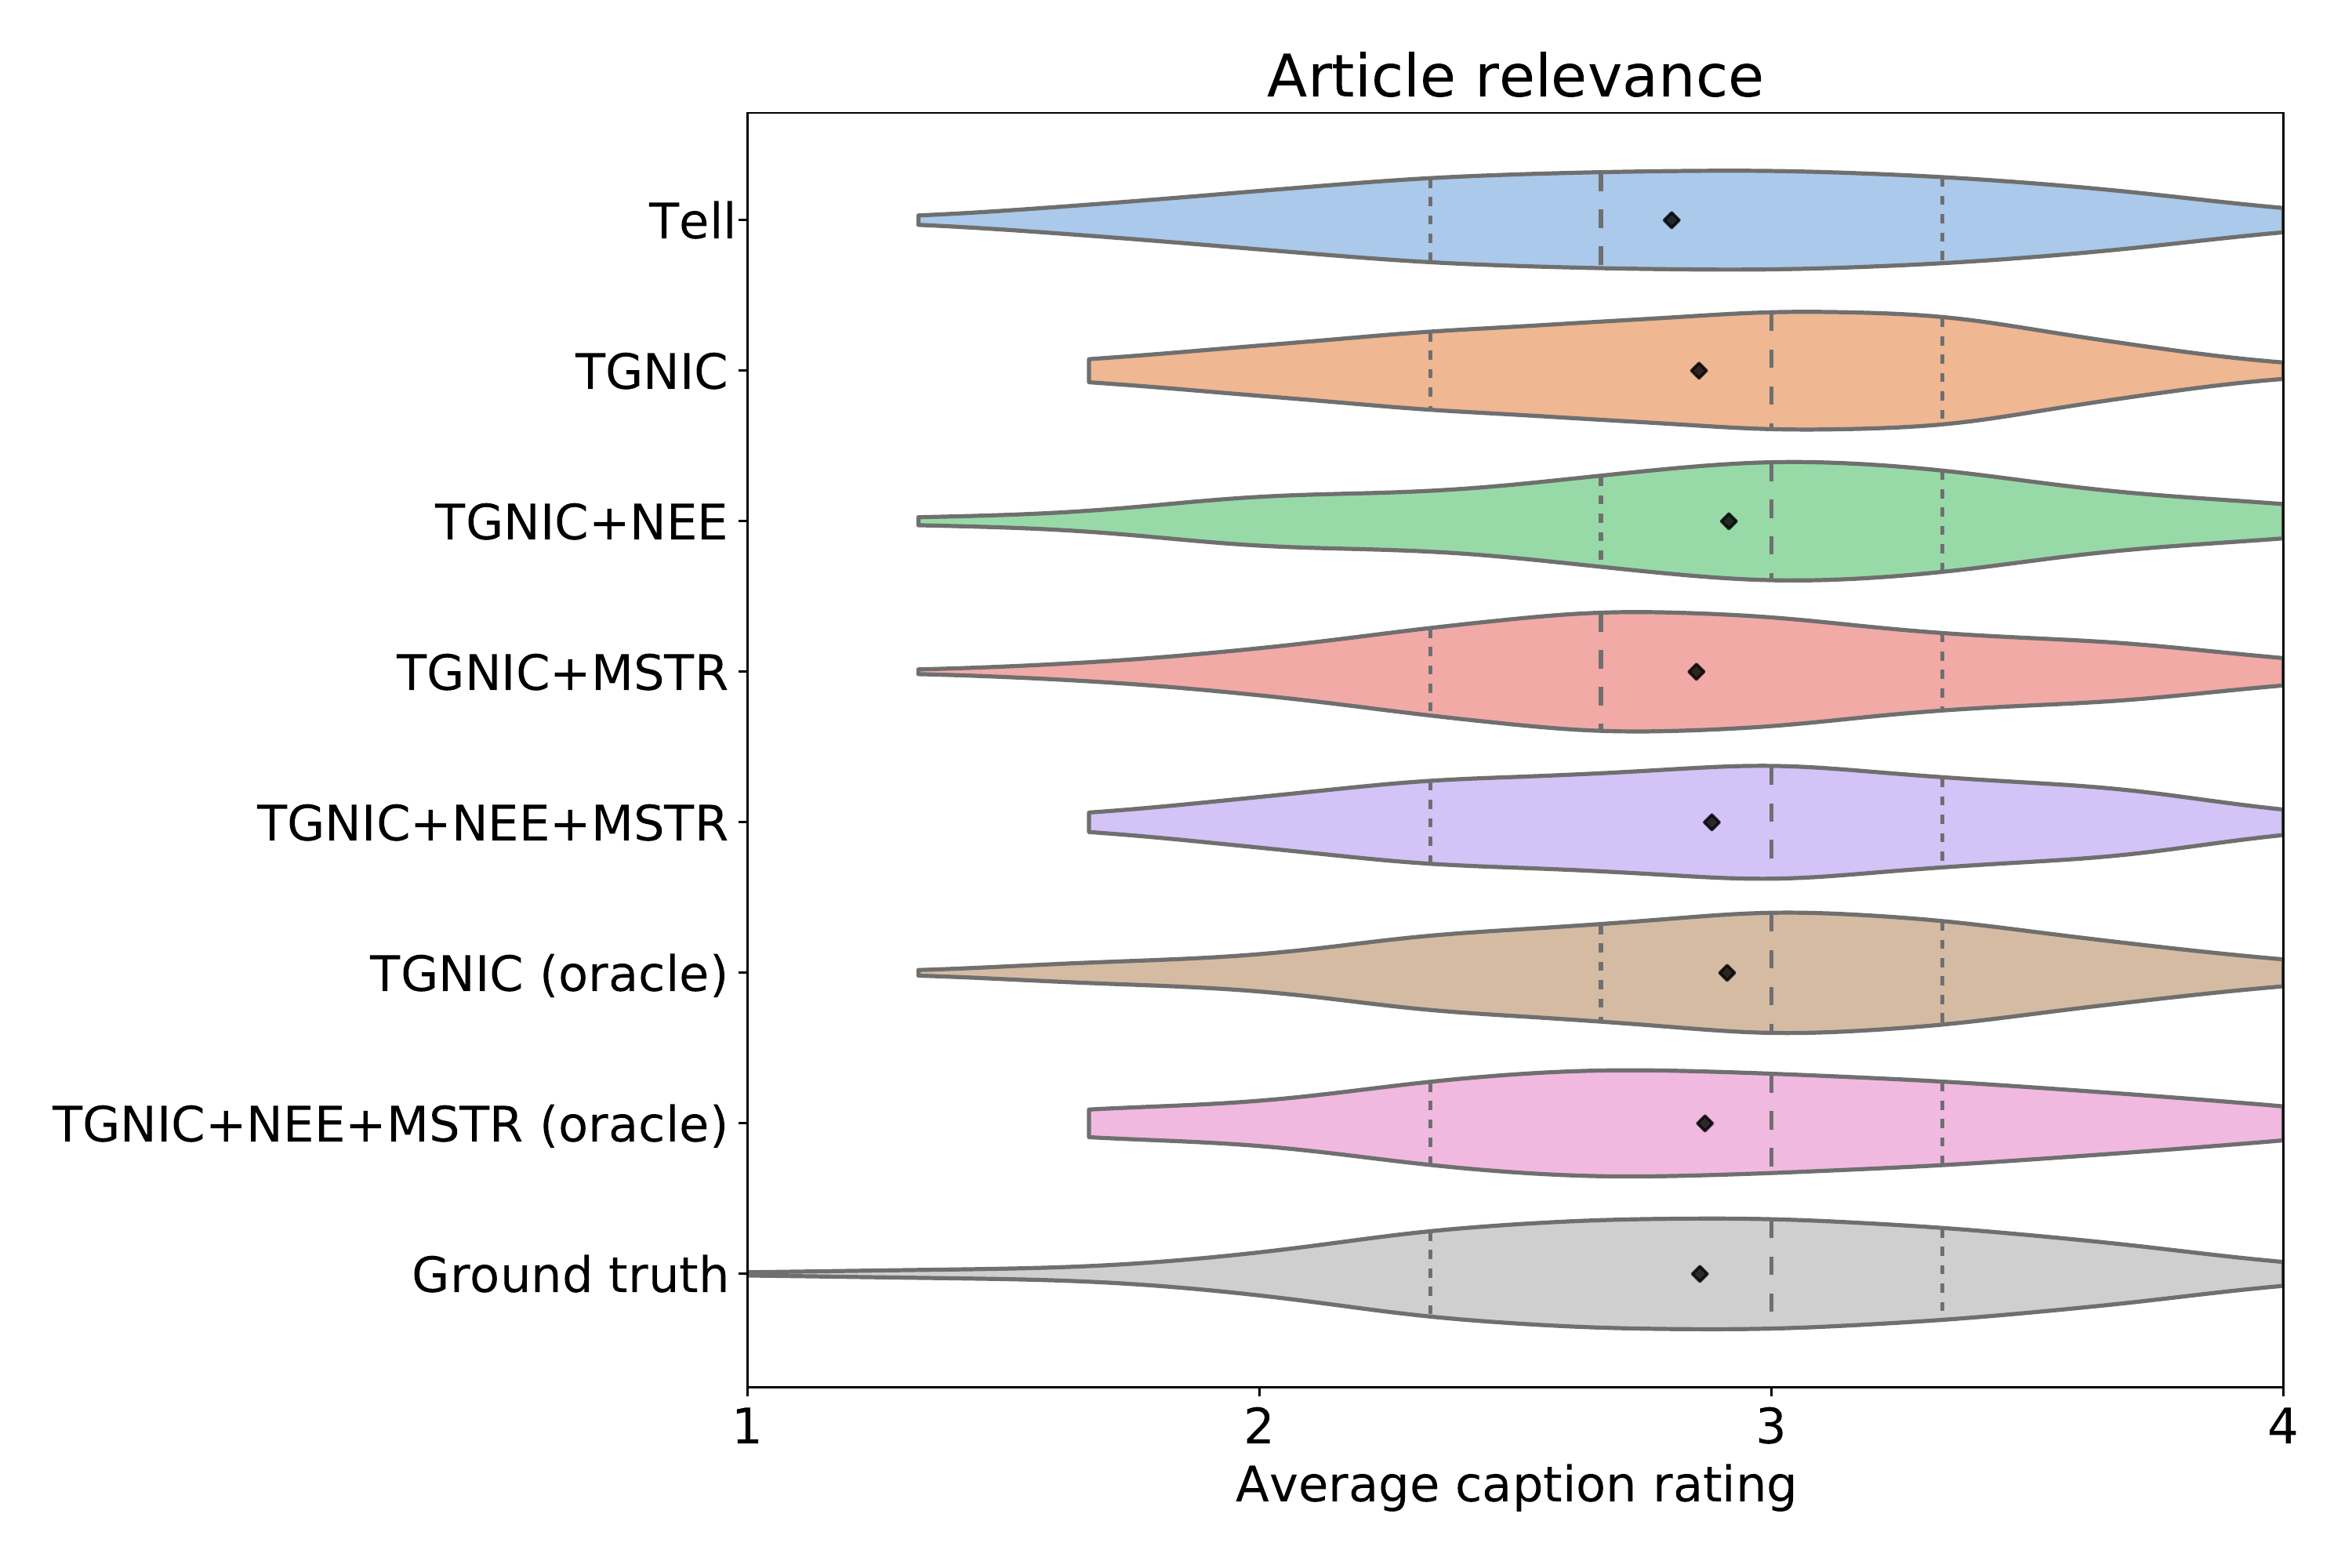}
%          \caption{Article relevance}
%          \label{fig:humaneval_art}
%      \end{subfigure}
%      \hfill
%      \begin{subfigure}[b]{0.3\textwidth}
%          \centering
%          \includegraphics[width=\textwidth]{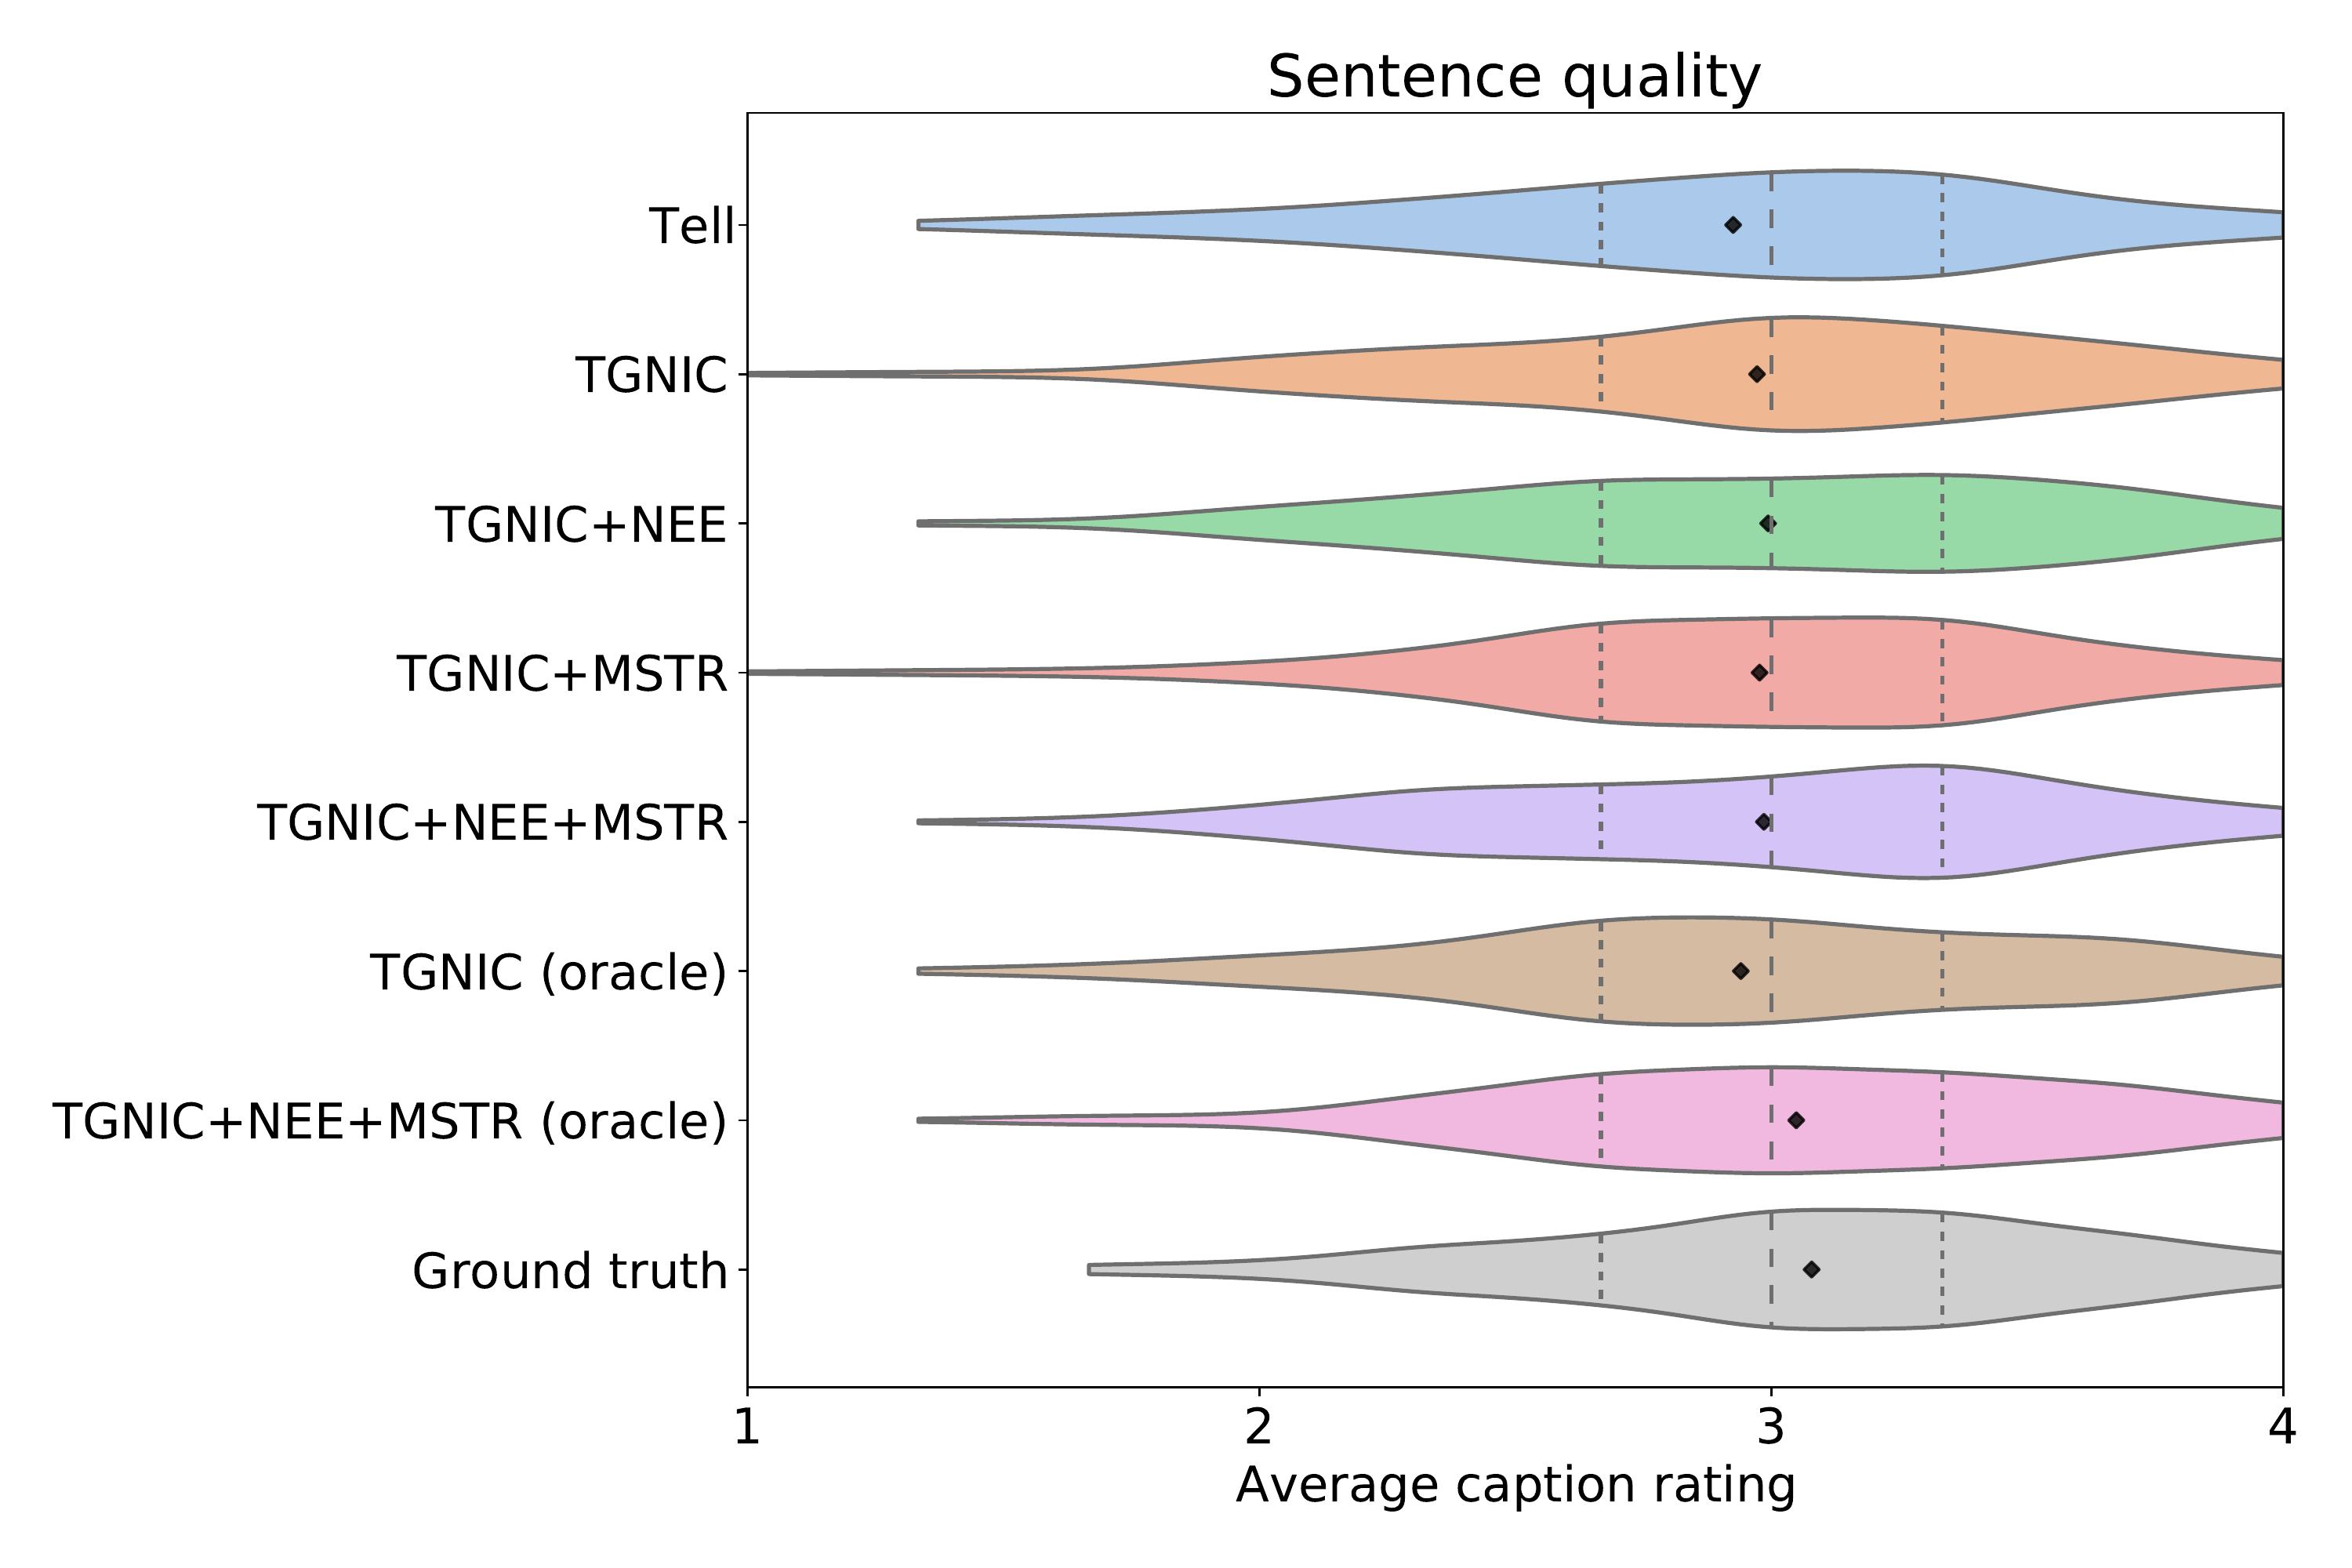}
%          \caption{Sentence quality}
%          \label{fig:humaneval_img}
%      \end{subfigure}
%         \caption{Human evaluation results.}
%         \label{fig:human_eval}
% \end{figure*}

\section{Ablation Study}
\begin{table*}[t]
\small
	\centering
	\begin{adjustbox}{max width=\textwidth}
	\begin{tabular}{cc|cccc|cc|c}
		%\toprule
		\cmidrule{3-9}
% 		 &
% 		 & \multirow{2}{*}{\textbf{\small{BLEU-4}}}
% 		 & \multirow{2}{*}{\textbf{\small{ROUGE}}}
% 		 & \multirow{2}{*}{\textbf{\small{METEOR}}}
% 		 & \multirow{2}{*}{\textbf{\small{CIDEr}}}
         & & \multicolumn{4}{c|}{\centering\textbf{\small{General Caption Ceneration}}}
		 & \multicolumn{2}{c|}{\textbf{\small{Named Entities}}} 
		 & \textbf{\small{Training Time}}
        \\
		 \cmidrule{3-9}
		 &  & \small{BLEU-4} & \small{ROUGE} & \small{METEOR} & \small{CIDEr} & \small{$P$} & \small{$R$} & \small{$h$/epoch}  \\
		\midrule
		%\multirow{12}{*}{\rotatebox[origin=c]{90}{GoodNews}}
		\multirow{6}{*}{\good}
		 & \name (Longformer) & 5.69 & 21.08 & 9.97 & 52.04 & 24.63 & 19.63 & \textbf{0.91} \\
		 & \name (RoBERTa) & 6.34 & 21.65 & 10.78 & 59.19 & 24.60 & 20.90 & 1.02 \\
		 & \name (RoBERTa+MSTR 800) & 6.38 & 21.72 & 10.80 & 59.33 & 24.63 & 21.22 & 1.23 \\
		 & \name (RoBERTa+MSTR 1000) & \textbf{6.45} & \textbf{21.99} & 10.83 & 59.65 & \textbf{24.75} & 21.61 & 1.41 \\
		 & \name (RoBERTa+MSTR 1200) & 6.44 & 21.98 & \textbf{10.85} & 59.66 & 24.74 & \textbf{21.63} & 1.58 \\
		 & \name (RoBERTa+MSTR 1400) & 6.45 & 21.96 & 10.80 & \textbf{59.67} & 24.74 & 21.60 & 1.83 \\
		\midrule
		\midrule
		\multirow{6}{*}{{\nyt}}
% 		 \cmidrule{2-8}
		 & \name (Longformer) & 5.72 & 19.55 & 9.87 & 41.66 & 22.89 & 18.09 & \textbf{0.94} \\
		 & \name (RoBERTa) & 6.39 & 22.38 & 10.75 & 56.54 & \textbf{27.35} & \textbf{23.73} & 1.09  \\
		 & \name (RoBERTa+MSTR 800) & 6.41 & 22.40 & 10.79 & 56.92 & 27.01 & 23.70 & 1.26 \\
		 & \name (RoBERTa+MSTR 1000) & \textbf{6.44} & 22.63 & \textbf{10.88} & \textbf{57.61} & 26.41 & 23.67 & 1.47 \\
		 & \name (RoBERTa+MSTR 1200) & 6.42 & \textbf{22.64} & 10.83 & 57.59 & 26.43 & 23.61 & 1.69 \\
		 & \name (RoBERTa+MSTR 1400) & 6.42 & 22.62 & 10.81 & 57.60 & 26.40 & 23.58 & 1.88 \\
		\bottomrule
	\end{tabular}
	\end{adjustbox}
	\caption {Results on \good and \nyt. We highlight the \textbf{best} model in bold.
	Note that we report the mean values of three runs, and the maximum standard derivations of our variants on BLEU, ROUGE, METEOR, CIDEr are 0.013, 0.019, 0.016 and 0.069, which shows the stability of our results and that our method improvements are notable.
	\label{tab:ablation_results}}
% 	\vspace{-0.3cm}
\end{table*}
% In addition to the main paper modality ablation results where, at test-time, we present image-only (zero-out article features) and text-only (zero-out image features), we further evaluate how each modality contribute to the \name, when we start training from scratch with one modality being zeroed-out.
% We have similar conclusion as in the main paper that both modality - image and article, contribute significantly to the final performance of \name.
In addition to the \textit{Multi-Span Text Reading} (MSTR) method proposed as an efficient technique to read long articles, we also try out Longformer~\cite{Longformer}, which is proposed to read long articles efficiently with an attention mechanism that scales linearly with sequence length.  
This attention mechanism is a drop-in replacement for the standard self-attention and combines a local windowed attention with a task motivated global attention.
In this experiment, we replace RoBERTa with Longformer as the text feature extractor. Results are shown in Tab.~\ref{tab:ablation_results}.
Unexpectedly, the Longformer variant of \name underperforms the RoBERTa variant.
The possible reason is that in order to improve training efficiency, Longformer applies local windowed attentions with sparse global attentions.
However, in this task, global attention is needed in every token.
One possible solution for Longformer is to re-do the pretraining with fully global attention. However, this might be a non-trivial task and we will explore this in the future work.

We also conduct experiments to get the best possible number of tokens for MSTR.
We applied number of tokens equal to $512$, $800$, $1000$, $1200$ and $1400$ respectively.
We found that the best choice is $1000$ as it provides nearly the best performance while the training time per epoch is still good enough.
